# Supplementary material for: Re-parameterizing VAEs for stability
Source: arXiv:2106.13739 source file (2021-06-25)
Supplement: Supplementary file 1 [file appendix.tex]

\newpage
\appendix

\section{Stability measurements on overfitted datasets}

We calculate a running mean $\mu_n$ and variance $v_n$, of the loss $l_n$, initially set to 0 and 1 with:

\begin{align}
\mu_{n+1} &= \epsilon*\mu_n+(1-\epsilon)*l_n \\
v_{n+1} &= \delta*v_n+(1-\delta)*(l_n-\mu_{n+1})^2
\end{align}
with $\epsilon=0.998$ and $\delta=0.9995$.

The Z score is then $Z_n=\frac{l_n-\mu_n}{\sqrt{v_n}}$.
A step $n$ is considered to be part of an instability if $Z > 4$ (Notice that we consider only positive anomalies).

As metrics we consider:
\begin{itemize}
    \item The proportion of experiments that returned \emph{Nan} or did not reach loss below -3000. (The latter ones correspond to the optimizer crashing).
    \item The minimal smooth loss attained.
    \item The proportion of steps in instabilities. This does not take peak height into account.
    \item The average value of $max(0, Z-4)$. This attempts to take peak height into account.
\end{itemize}

\begin{table}%
\centering%
\adjustbox{tabular=|c|c|c|c|c|c|c|c|, center}{
\hline%
lr&Architecture&\multicolumn{6}{|c|}{Parametrization}\\%
\hline%
&&Vanilla&Exp&ExpLin&UpBounded&InverseLin&LogInverseLin\\%
\hline%
\multirow{3}{*}{0.008}&Basic&{-}&{-}&$-7624 \pm 324$&$-7488 \pm 391$&$-7294 \pm 175$&$-7305 \pm 247$\\%
~&Sep. Paths&{-}&{-}&$-7345 \pm 328$&$-7622 \pm 179$&$-7489 \pm 287$&$-7184 \pm 283$\\%
~&Sigma Global&$-7514 \pm 372$&$-7561 \pm 280$&$-7494 \pm 331$&$-7509 \pm 478$&$-7423 \pm 207$&$-7036 \pm 351$\\%
\hline%
\multirow{3}{*}{0.007}&Basic&{-}&{-}&$-7657 \pm 323$&$-7682 \pm 329$&$-7617 \pm 245$&$-7669 \pm 295$\\%
~&Sep. Paths&{-}&{-}&$-7681 \pm 222$&$-7756 \pm 193$&$-7691 \pm 308$&$-7550 \pm 460$\\%
~&Sigma Global&$-7573 \pm 288$&$-7598 \pm 404$&$-7591 \pm 225$&$-7552 \pm 281$&$-7579 \pm 226$&$-7357 \pm 287$\\%
\hline%
\multirow{3}{*}{0.006}&Basic&{-}&{-}&$-8024 \pm 171$&$-7852 \pm 283$&$-7891 \pm 324$&$-7779 \pm 229$\\%
~&Sep. Paths&{-}&$-7596 \pm 304$&$-7767 \pm 404$&$-7844 \pm 388$&$-7748 \pm 220$&$-7728 \pm 283$\\%
~&Sigma Global&$-7848 \pm 222$&$-7724 \pm 325$&$-7803 \pm 349$&$-7927 \pm 329$&$-7737 \pm 207$&$-7458 \pm 302$\\%
\hline%
}
\caption{Minimal smoothed loss attained}%
\end{table}

\begin{table}%
\centering%
\adjustbox{tabular=|c|c|c|c|c|c|c|c|, center}{
\hline%
lr&Architecture&\multicolumn{6}{|c|}{Parametrization}\\%
\hline%
&&Vanilla&Exp&ExpLin&UpBounded&InverseLin&LogInverseLin\\%
\hline%
\multirow{3}{*}{0.008}&Basic&10 / 10&6 / 10&0 / 10&0 / 10&0 / 10&0 / 10\\%
~&Sep. Paths&10 / 10&9 / 10&0 / 10&0 / 10&0 / 10&0 / 10\\%
~&Sigma Global&0 / 10&0 / 10&0 / 10&0 / 10&0 / 10&0 / 10\\%
\hline%
\multirow{3}{*}{0.007}&Basic&10 / 10&7 / 10&0 / 10&0 / 10&0 / 10&0 / 10\\%
~&Sep. Paths&9 / 10&7 / 10&0 / 10&0 / 10&0 / 10&0 / 10\\%
~&Sigma Global&0 / 10&0 / 10&0 / 10&0 / 10&0 / 10&0 / 10\\%
\hline%
\multirow{3}{*}{0.006}&Basic&2 / 10&2 / 10&0 / 10&0 / 10&0 / 10&0 / 10\\%
~&Sep. Paths&2 / 10&0 / 10&0 / 10&0 / 10&0 / 10&0 / 10\\%
~&Sigma Global&0 / 10&0 / 10&0 / 10&0 / 10&0 / 10&0 / 10\\%
\hline%
}
\caption{Proportion of runs that returned \emph{Nan} output or did not attain loss below -3000}%
\end{table}

\begin{table}%
\centering%
\adjustbox{tabular=|c|c|c|c|c|c|c|c|, center}{
\hline%
lr&Architecture&\multicolumn{6}{|c|}{Parametrization}\\%
\hline%
&&Vanilla&Exp&ExpLin&UpBounded&InverseLin&LogInverseLin\\%
\hline%
\multirow{3}{*}{0.008}&Basic&{-}&{-}&$0.027 \pm 0.023$&$0.034 \pm 0.016$&$0.039 \pm 0.047$&$0.030 \pm 0.023$\\%
~&Sep. Paths&{-}&{-}&$0.033 \pm 0.014$&$0.035 \pm 0.014$&$0.040 \pm 0.022$&$0.068 \pm 0.036$\\%
~&Sigma Global&$0.021 \pm 0.011$&$0.031 \pm 0.014$&$0.026 \pm 0.012$&$0.018 \pm 0.010$&$0.028 \pm 0.012$&$0.010 \pm 0.009$\\%
\hline%
\multirow{3}{*}{0.007}&Basic&{-}&{-}&$0.017 \pm 0.012$&$0.022 \pm 0.014$&$0.030 \pm 0.027$&$0.015 \pm 0.013$\\%
~&Sep. Paths&{-}&{-}&$0.026 \pm 0.020$&$0.023 \pm 0.015$&$0.030 \pm 0.013$&$0.094 \pm 0.043$\\%
~&Sigma Global&$0.017 \pm 0.008$&$0.020 \pm 0.011$&$0.021 \pm 0.011$&$0.022 \pm 0.011$&$0.016 \pm 0.010$&$0.010 \pm 0.009$\\%
\hline%
\multirow{3}{*}{0.006}&Basic&{-}&{-}&$0.017 \pm 0.015$&$0.008 \pm 0.007$&$0.018 \pm 0.016$&$0.008 \pm 0.006$\\%
~&Sep. Paths&{-}&$0.008 \pm 0.009$&$0.017 \pm 0.012$&$0.024 \pm 0.021$&$0.014 \pm 0.013$&$0.056 \pm 0.026$\\%
~&Sigma Global&$0.018 \pm 0.014$&$0.012 \pm 0.010$&$0.014 \pm 0.007$&$0.016 \pm 0.015$&$0.011 \pm 0.010$&$0.002 \pm 0.001$\\%
\hline%
}
\caption{Proportion of iteration spent in an instability.}%
\end{table}

\begin{table}%
\centering%
\adjustbox{tabular=|c|c|c|c|c|c|c|c|, center}{
\hline%
lr&Architecture&\multicolumn{6}{|c|}{Parametrization}\\%
\hline%
&&Vanilla&Exp&ExpLin&UpBounded&InverseLin&LogInverseLin\\%
\hline%
\multirow{3}{*}{0.008}&Basic&{-}&{-}&$0.168 \pm 0.246$&$0.225 \pm 0.140$&$0.330 \pm 0.544$&$0.230 \pm 0.203$\\%
~&Sep. Paths&{-}&{-}&$0.221 \pm 0.136$&$0.200 \pm 0.141$&$0.274 \pm 0.335$&$1.001 \pm 1.042$\\%
~&Sigma Global&$0.156 \pm 0.158$&$0.168 \pm 0.080$&$0.124 \pm 0.065$&$0.143 \pm 0.130$&$0.218 \pm 0.134$&$0.086 \pm 0.105$\\%
\hline%
\multirow{3}{*}{0.007}&Basic&{-}&{-}&$0.102 \pm 0.096$&$0.119 \pm 0.087$&$0.237 \pm 0.315$&$0.113 \pm 0.128$\\%
~&Sep. Paths&{-}&{-}&$0.141 \pm 0.149$&$0.114 \pm 0.117$&$0.172 \pm 0.105$&$0.614 \pm 0.338$\\%
~&Sigma Global&$0.112 \pm 0.114$&$0.158 \pm 0.105$&$0.164 \pm 0.116$&$0.126 \pm 0.069$&$0.112 \pm 0.114$&$0.060 \pm 0.079$\\%
\hline%
\multirow{3}{*}{0.006}&Basic&{-}&{-}&$0.099 \pm 0.115$&$0.036 \pm 0.051$&$0.095 \pm 0.115$&$0.038 \pm 0.051$\\%
~&Sep. Paths&{-}&$0.024 \pm 0.029$&$0.074 \pm 0.085$&$0.161 \pm 0.246$&$0.107 \pm 0.157$&$0.318 \pm 0.195$\\%
~&Sigma Global&$0.103 \pm 0.100$&$0.059 \pm 0.059$&$0.077 \pm 0.054$&$0.077 \pm 0.083$&$0.053 \pm 0.077$&$0.003 \pm 0.002$\\%
\hline%
}
\caption{Mean value of max(Z-4, 0) where Z is the standard Z score measured with the smoothed mean and std values}%
\end{table}

\section{Effect of maximum in UpBounded}

\begin{table}%
\centering%
\adjustbox{tabular=|c|c|c|c|c|c|, center}{
\hline%
lr&Architecture&\multicolumn{4}{|c|}{Parametrization}\\%
\hline%
&&C=0.5&C=1.&C=1.5&C=2.\\%
\hline%
\multirow{1}{*}{0.008}&Basic&$-7565 \pm 229$&$-7329 \pm 288$&$-7430 \pm 269$&$-7488 \pm 391$\\%
\hline%
\multirow{1}{*}{0.007}&Basic&$-7617 \pm 263$&$-7526 \pm 147$&$-7559 \pm 233$&$-7682 \pm 329$\\%
\hline%
\multirow{1}{*}{0.006}&Basic&$-7612 \pm 293$&$-7911 \pm 368$&$-7827 \pm 199$&$-7852 \pm 283$\\%
\hline%
}
\caption{Minimal smoothed loss attained}%
\end{table}

\begin{table}%
\centering%
\adjustbox{tabular=|c|c|c|c|c|c|, center}{
\hline%
lr&Architecture&\multicolumn{4}{|c|}{Parametrization}\\%
\hline%
&&C=0.5&C=1.&C=1.5&C=2.\\%
\hline%
\multirow{1}{*}{0.008}&Basic&0 / 10&0 / 10&0 / 10&0 / 10\\%
\hline%
\multirow{1}{*}{0.007}&Basic&0 / 10&0 / 10&0 / 10&0 / 10\\%
\hline%
\multirow{1}{*}{0.006}&Basic&0 / 10&0 / 10&0 / 10&0 / 10\\%
\hline%
}
\caption{Proportion of runs that returned \emph{Nan} output or did not attain loss below -3000}%
\end{table}

\begin{table}%
\centering%
\adjustbox{tabular=|c|c|c|c|c|c|, center}{
\hline%
lr&Architecture&\multicolumn{4}{|c|}{Parametrization}\\%
\hline%
&&C=0.5&C=1.&C=1.5&C=2.\\%
\hline%
\multirow{1}{*}{0.008}&Basic&$0.031 \pm 0.018$&$0.020 \pm 0.012$&$0.027 \pm 0.028$&$0.034 \pm 0.016$\\%
\hline%
\multirow{1}{*}{0.007}&Basic&$0.021 \pm 0.017$&$0.020 \pm 0.015$&$0.019 \pm 0.016$&$0.022 \pm 0.014$\\%
\hline%
\multirow{1}{*}{0.006}&Basic&$0.010 \pm 0.009$&$0.015 \pm 0.014$&$0.009 \pm 0.006$&$0.008 \pm 0.007$\\%
\hline%
}
\caption{Proportion of iteration spent in an instability.}%
\end{table}

\begin{table}%
\centering%
\adjustbox{tabular=|c|c|c|c|c|c|, center}{
\hline%
lr&Architecture&\multicolumn{4}{|c|}{Parametrization}\\%
\hline%
&&C=0.5&C=1.&C=1.5&C=2.\\%
\hline%
\multirow{1}{*}{0.008}&Basic&$0.169 \pm 0.119$&$0.134 \pm 0.129$&$0.221 \pm 0.245$&$0.225 \pm 0.140$\\%
\hline%
\multirow{1}{*}{0.007}&Basic&$0.098 \pm 0.083$&$0.113 \pm 0.109$&$0.164 \pm 0.170$&$0.119 \pm 0.087$\\%
\hline%
\multirow{1}{*}{0.006}&Basic&$0.054 \pm 0.058$&$0.103 \pm 0.106$&$0.058 \pm 0.048$&$0.036 \pm 0.051$\\%
\hline%
}
\caption{Mean value of max(Z-4, 0) where Z is the standard Z score measured with the smoothed mean and std values}%
\end{table}

\section{Bounded parametrisation}
\begin{table}%
\centering%
\adjustbox{tabular=|c|c|c|c|c|c|, center}{
\hline%
lr&Architecture&\multicolumn{4}{|c|}{Parametrization}\\%
\hline%
&&LowerUpBounded 1e{-}4&UpBounded 1e{-}4, 1&BoundedLin  1e{-}4, 1&BoundedLogLin  1e{-}4, 1\\%
\hline%
\multirow{3}{*}{0.008}&Basic&($-1129 \pm 2134$)&$-7449 \pm 287$&$-7522 \pm 238$&$-7308 \pm 249$\\%
~&Sep. Paths.&($-4924 \pm 2547$)&$-6504 \pm 347$&$-7489 \pm 268$&$-7434 \pm 153$\\%
~&Sigma Global&$-7660 \pm 350$&$-7431 \pm 232$&$-7702 \pm 179$&$-7347 \pm 198$\\%
\hline%
\multirow{3}{*}{0.007}&Basic&($-3999 \pm 3445$)&$-7486 \pm 297$&$-7509 \pm 345$&$-7547 \pm 284$\\%
~&Sep. Paths.&($-5152 \pm 2697$)&$-6532 \pm 281$&$-7513 \pm 331$&$-7560 \pm 304$\\%
~&Sigma Global&$-7629 \pm 326$&$-7598 \pm 219$&$-7717 \pm 264$&$-7328 \pm 286$\\%
\hline%
\multirow{3}{*}{0.006}&Basic&$-7426 \pm 1006$&$-7674 \pm 285$&$-7760 \pm 265$&$-7666 \pm 246$\\%
~&Sep. Paths.&($-6999 \pm 1982$)&$-6482 \pm 291$&$-7726 \pm 89$&$-7621 \pm 310$\\%
~&Sigma Global&$-7807 \pm 244$&$-7869 \pm 277$&$-7829 \pm 283$&$-7511 \pm 268$\\%
\hline%
}
\caption{Minimal smoothed loss attained}%
\end{table}

\begin{table}%
\centering%
\adjustbox{tabular=|c|c|c|c|c|c|, center}{
\hline%
lr&Architecture&\multicolumn{4}{|c|}{Parametrization}\\%
\hline%
&&LowerUpBounded 1e{-}4&UpBounded 1e{-}4, 1&BoundedLin  1e{-}4, 1&BoundedLogLin  1e{-}4, 1\\%
\hline%
\multirow{3}{*}{0.008}&Basic&7 / 10&0 / 10&0 / 10&0 / 10\\%
~&Sep. Paths.&7 / 10&0 / 10&0 / 10&0 / 10\\%
~&Sigma Global&0 / 10&0 / 10&0 / 10&0 / 10\\%
\hline%
\multirow{3}{*}{0.007}&Basic&4 / 10&0 / 10&0 / 10&0 / 10\\%
~&Sep. Paths.&7 / 10&0 / 10&0 / 10&0 / 10\\%
~&Sigma Global&0 / 10&0 / 10&0 / 10&0 / 10\\%
\hline%
\multirow{3}{*}{0.006}&Basic&0 / 10&0 / 10&0 / 10&0 / 10\\%
~&Sep. Paths.&2 / 10&0 / 10&0 / 10&0 / 10\\%
~&Sigma Global&0 / 10&0 / 10&0 / 10&0 / 10\\%
\hline%
}
\caption{Proportion of runs that returned \emph{Nan} output or did not attain loss below -3000}%
\end{table}

\begin{table}%
\centering%
\adjustbox{tabular=|c|c|c|c|c|c|, center}{
\hline%
lr&Architecture&\multicolumn{4}{|c|}{Parametrization}\\%
\hline%
&&LowerUpBounded 1e{-}4&UpBounded 1e{-}4, 1&BoundedLin  1e{-}4, 1&BoundedLogLin  1e{-}4, 1\\%
\hline%
\multirow{3}{*}{0.008}&Basic&($0.004 \pm 0.006$)&$0.032 \pm 0.019$&$0.032 \pm 0.024$&$0.027 \pm 0.021$\\%
~&Sep. Paths.&($0.025 \pm 0.074$)&$0.004 \pm 0.006$&$0.029 \pm 0.015$&$0.028 \pm 0.012$\\%
~&Sigma Global&$0.036 \pm 0.014$&$0.021 \pm 0.015$&$0.030 \pm 0.015$&$0.018 \pm 0.012$\\%
\hline%
\multirow{3}{*}{0.007}&Basic&($0.021 \pm 0.029$)&$0.017 \pm 0.014$&$0.016 \pm 0.012$&$0.013 \pm 0.013$\\%
~&Sep. Paths.&($0.096 \pm 0.266$)&$0.002 \pm 0.001$&$0.019 \pm 0.013$&$0.020 \pm 0.018$\\%
~&Sigma Global&$0.021 \pm 0.021$&$0.015 \pm 0.011$&$0.022 \pm 0.017$&$0.011 \pm 0.012$\\%
\hline%
\multirow{3}{*}{0.006}&Basic&$0.072 \pm 0.169$&$0.012 \pm 0.006$&$0.015 \pm 0.013$&$0.009 \pm 0.010$\\%
~&Sep. Paths.&($0.017 \pm 0.014$)&$0.002 \pm 0.001$&$0.012 \pm 0.011$&$0.008 \pm 0.007$\\%
~&Sigma Global&$0.013 \pm 0.013$&$0.016 \pm 0.010$&$0.011 \pm 0.010$&$0.007 \pm 0.005$\\%
\hline%
}
\caption{Proportion of iteration spent in an instability.}%
\end{table}

\begin{table}%
\centering%
\adjustbox{tabular=|c|c|c|c|c|c|, center}{
\hline%
lr&Architecture&\multicolumn{4}{|c|}{Parametrization}\\%
\hline%
&&LowerUpBounded 1e{-}4&UpBounded 1e{-}4, 1&BoundedLin  1e{-}4, 1&BoundedLogLin  1e{-}4, 1\\%
\hline%
\multirow{3}{*}{0.008}&Basic&($inf \pm nan$)&$0.258 \pm 0.188$&$0.185 \pm 0.156$&$0.253 \pm 0.300$\\%
~&Sep. Paths.&($inf \pm nan$)&$0.026 \pm 0.071$&$0.183 \pm 0.088$&$0.167 \pm 0.094$\\%
~&Sigma Global&$0.231 \pm 0.134$&$0.117 \pm 0.113$&$0.163 \pm 0.108$&$0.104 \pm 0.103$\\%
\hline%
\multirow{3}{*}{0.007}&Basic&($inf \pm nan$)&$0.079 \pm 0.070$&$0.114 \pm 0.098$&$0.077 \pm 0.111$\\%
~&Sep. Paths.&($inf \pm nan$)&$0.002 \pm 0.002$&$0.134 \pm 0.119$&$0.174 \pm 0.207$\\%
~&Sigma Global&$0.103 \pm 0.123$&$0.096 \pm 0.095$&$0.147 \pm 0.128$&$0.080 \pm 0.101$\\%
\hline%
\multirow{3}{*}{0.006}&Basic&$16530081.405 \pm 49590239.532$&$0.054 \pm 0.041$&$0.091 \pm 0.076$&$0.051 \pm 0.079$\\%
~&Sep. Paths.&($107044136550.518 \pm 321132409651.161$)&$0.002 \pm 0.002$&$0.059 \pm 0.076$&$0.058 \pm 0.082$\\%
~&Sigma Global&$0.081 \pm 0.113$&$0.122 \pm 0.115$&$0.067 \pm 0.083$&$0.051 \pm 0.106$\\%
\hline%
}
\caption{Mean value of max(Z-4, 0) where Z is the standard Z score measured with the smoothed mean and std values}%
\end{table}

\section{C2 version of parametrization in latent space}

\begin{table}%
\centering%
\adjustbox{tabular=|c|c|c|c|c|, center}{
\hline%
lr&Architecture&\multicolumn{3}{|c|}{Parametrization}\\%
\hline%
&&C2 Bounded&C2 explin&Bounded Exp.\\%
\hline%
\multirow{1}{*}{0.008}&Basic&$-7511 \pm 268$&$-7393 \pm 221$&$-7488 \pm 391$\\%
\hline%
}
\caption{Minimal smoothed loss attained}%
\end{table}

\begin{table}%
\centering%
\adjustbox{tabular=|c|c|c|c|c|, center}{
\hline%
lr&Architecture&\multicolumn{3}{|c|}{Parametrization}\\%
\hline%
&&C2 Bounded&C2 explin&Bounded Exp.\\%
\hline%
\multirow{1}{*}{0.008}&Basic&0 / 10&0 / 10&0 / 10\\%
\hline%
}
\caption{Proportion of runs that returned \emph{Nan} output or did not attain loss below -3000}%
\end{table}

\begin{table}%
\centering%
\adjustbox{tabular=|c|c|c|c|c|, center}{
\hline%
lr&Architecture&\multicolumn{3}{|c|}{Parametrization}\\%
\hline%
&&C2 Bounded&C2 explin&Bounded Exp.\\%
\hline%
\multirow{1}{*}{0.008}&Basic&$0.044 \pm 0.018$&$0.028 \pm 0.009$&$0.034 \pm 0.016$\\%
\hline%
}
\caption{Proportion of iteration spent in an instability.}%
\end{table}

\begin{table}%
\centering%
\adjustbox{tabular=|c|c|c|c|c|, center}{
\hline%
lr&Architecture&\multicolumn{3}{|c|}{Parametrization}\\%
\hline%
&&C2 Bounded&C2 explin&Bounded Exp.\\%
\hline%
\multirow{1}{*}{0.008}&Basic&$0.252 \pm 0.147$&$0.221 \pm 0.089$&$0.225 \pm 0.140$\\%
\hline%
}
\caption{Mean value of max(Z-4, 0) where Z is the standard Z score measured with the smoothed mean and std values}%
\end{table}

\section{Parametrized sigma decoded}

\begin{table}%
\centering%
\adjustbox{tabular=|c|c|c|c|c|, center}{
\hline%
lr&$\gamma$-Parametrization&\multicolumn{3}{|c|}{$\sigma$ Parametrization}\\%
\hline%
&&Vanilla&Exp&UpBounded\\%
\hline%
\multirow{3}{*}{0.008}&Vanilla&($0 \pm 0$)&($-713 \pm 2141$)&$-7729 \pm 321$\\%
~&Exp&($-775 \pm 2327$)&($-2221 \pm 3394$)&$-7729 \pm 218$\\%
~&UpBounded&($-758 \pm 2274$)&($-865 \pm 2295$)&$-7870 \pm 112$\\%
\hline%
\multirow{3}{*}{0.007}&Vanilla&($-2340 \pm 3576$)&($-2339 \pm 3576$)&$-7971 \pm 253$\\%
~&Exp&($-3983 \pm 3985$)&($-6111 \pm 3065$)&$-7830 \pm 305$\\%
~&UpBounded&($-3159 \pm 3872$)&($-4663 \pm 3816$)&$-7508 \pm 247$\\%
\hline%
\multirow{3}{*}{0.006}&Vanilla&($-6349 \pm 3180$)&$-7855 \pm 250$&$-8035 \pm 252$\\%
~&Exp&$-7954 \pm 343$&$-8000 \pm 196$&$-7782 \pm 227$\\%
~&UpBounded&($-6518 \pm 3225$)&$-7681 \pm 293$&$-7785 \pm 332$\\%
\hline%
}
\caption{Minimal smoothed loss attained}%
\end{table}

\begin{table}%
\centering%
\adjustbox{tabular=|c|c|c|c|c|, center}{
\hline%
lr&$\gamma$-Parametrization&\multicolumn{3}{|c|}{$\sigma$ Parametrization}\\%
\hline%
&&Vanilla&Exp&UpBounded\\%
\hline%
\multirow{3}{*}{0.008}&Vanilla&10 / 10&10 / 10&0 / 10\\%
~&Exp&9 / 10&7 / 10&0 / 10\\%
~&UpBounded&9 / 10&9 / 10&0 / 10\\%
\hline%
\multirow{3}{*}{0.007}&Vanilla&8 / 10&7 / 10&0 / 10\\%
~&Exp&5 / 10&2 / 10&0 / 10\\%
~&UpBounded&7 / 10&5 / 10&0 / 10\\%
\hline%
\multirow{3}{*}{0.006}&Vanilla&3 / 10&0 / 10&0 / 10\\%
~&Exp&0 / 10&0 / 10&0 / 10\\%
~&UpBounded&2 / 10&0 / 10&0 / 10\\%
\hline%
}
\caption{Proportion of runs that returned \emph{Nan} output or did not attain loss below -3000}%
\end{table}

\begin{table}%
\centering%
\adjustbox{tabular=|c|c|c|c|c|, center}{
\hline%
lr&$\gamma$-Parametrization&\multicolumn{3}{|c|}{$\sigma$ Parametrization}\\%
\hline%
&&Vanilla&Exp&UpBounded\\%
\hline%
\multirow{3}{*}{0.008}&Vanilla&($0.000 \pm 0.000$)&($0.001 \pm 0.004$)&$0.007 \pm 0.004$\\%
~&Exp&($0.001 \pm 0.002$)&($0.000 \pm 0.001$)&$0.004 \pm 0.004$\\%
~&UpBounded&($0.003 \pm 0.009$)&($0.000 \pm 0.000$)&$0.005 \pm 0.003$\\%
\hline%
\multirow{3}{*}{0.007}&Vanilla&($0.001 \pm 0.001$)&($0.001 \pm 0.002$)&$0.004 \pm 0.001$\\%
~&Exp&($0.002 \pm 0.002$)&($0.002 \pm 0.001$)&$0.004 \pm 0.002$\\%
~&UpBounded&($0.001 \pm 0.002$)&($0.019 \pm 0.054$)&$0.003 \pm 0.002$\\%
\hline%
\multirow{3}{*}{0.006}&Vanilla&($0.003 \pm 0.003$)&$0.003 \pm 0.001$&$0.003 \pm 0.001$\\%
~&Exp&$0.003 \pm 0.001$&$0.005 \pm 0.003$&$0.003 \pm 0.002$\\%
~&UpBounded&($0.003 \pm 0.002$)&$0.003 \pm 0.002$&$0.004 \pm 0.002$\\%
\hline%
}
\caption{Proportion of iteration spent in an instability.}%
\end{table}

\begin{table}%
\centering%
\adjustbox{tabular=|c|c|c|c|c|, center}{
\hline%
lr&$\gamma$-Parametrization&\multicolumn{3}{|c|}{$\sigma$ Parametrization}\\%
\hline%
&&Vanilla&Exp&UpBounded\\%
\hline%
\multirow{3}{*}{0.008}&Vanilla&($0.000 \pm 0.000$)&($25.155 \pm 75.465$)&$0.042 \pm 0.045$\\%
~&Exp&($0.005 \pm 0.014$)&($0.000 \pm 0.001$)&$0.017 \pm 0.035$\\%
~&UpBounded&($0.028 \pm 0.083$)&($0.000 \pm 0.000$)&$0.013 \pm 0.017$\\%
\hline%
\multirow{3}{*}{0.007}&Vanilla&($inf \pm nan$)&($0.001 \pm 0.002$)&$0.007 \pm 0.006$\\%
~&Exp&($0.002 \pm 0.003$)&($0.003 \pm 0.002$)&$0.009 \pm 0.010$\\%
~&UpBounded&($0.062 \pm 0.181$)&($inf \pm nan$)&$0.011 \pm 0.015$\\%
\hline%
\multirow{3}{*}{0.006}&Vanilla&($0.068 \pm 0.194$)&$0.004 \pm 0.003$&$0.005 \pm 0.003$\\%
~&Exp&$0.008 \pm 0.013$&$0.016 \pm 0.022$&$0.007 \pm 0.010$\\%
~&UpBounded&($0.005 \pm 0.004$)&$0.005 \pm 0.008$&$0.006 \pm 0.006$\\%
\hline%
}
\caption{Mean value of max(Z-4, 0) where Z is the standard Z score measured with the smoothed mean and std values}%
\end{table}

\section{Parametrized global $\gamma$}

\begin{table}%
\centering%
\adjustbox{tabular=|c|c|c|c|c|, center}{
\hline%
lr&$\gamma$-Parametrization&\multicolumn{3}{|c|}{$\sigma$ Parametrization}\\%
\hline%
&&Vanilla&Exp&BoundedExp\\%
\hline%
\multirow{3}{*}{0.008}&Vanilla&($0 \pm 0$)&($-731 \pm 1462$)&$-7410 \pm 340$\\%
~&Exp&($0 \pm 0$)&($-2054 \pm 3138$)&$-7467 \pm 250$\\%
~&BoundedExp&($0 \pm 0$)&($-1420 \pm 2586$)&$-7566 \pm 313$\\%
\hline%
\multirow{3}{*}{0.007}&Vanilla&($0 \pm 0$)&($-4319 \pm 3534$)&$-7584 \pm 292$\\%
~&Exp&($-1607 \pm 2794$)&($-2835 \pm 3359$)&$-7477 \pm 259$\\%
~&BoundedExp&($-1639 \pm 3057$)&($-4942 \pm 3040$)&$-7572 \pm 273$\\%
\hline%
\multirow{3}{*}{0.006}&Vanilla&($-2438 \pm 3572$)&($-4516 \pm 3631$)&$-7526 \pm 295$\\%
~&Exp&($-809 \pm 2427$)&($-3028 \pm 3712$)&$-7692 \pm 246$\\%
~&BoundedExp&($-3791 \pm 3796$)&($-2300 \pm 3484$)&$-7765 \pm 390$\\%
\hline%
}
\caption{Minimal smoothed loss attained}%
\end{table}

\begin{table}%
\centering%
\adjustbox{tabular=|c|c|c|c|c|, center}{
\hline%
lr&$\gamma$-Parametrization&\multicolumn{3}{|c|}{$\sigma$ Parametrization}\\%
\hline%
&&Vanilla&Exp&BoundedExp\\%
\hline%
\multirow{3}{*}{0.008}&Vanilla&10 / 10&10 / 10&0 / 10\\%
~&Exp&10 / 10&7 / 10&0 / 10\\%
~&BoundedExp&10 / 10&8 / 10&0 / 10\\%
\hline%
\multirow{3}{*}{0.007}&Vanilla&10 / 10&4 / 10&0 / 10\\%
~&Exp&8 / 10&7 / 10&0 / 10\\%
~&BoundedExp&8 / 10&5 / 10&0 / 10\\%
\hline%
\multirow{3}{*}{0.006}&Vanilla&7 / 10&5 / 10&0 / 10\\%
~&Exp&9 / 10&6 / 10&0 / 10\\%
~&BoundedExp&5 / 10&7 / 10&0 / 10\\%
\hline%
}
\caption{Proportion of runs that returned \emph{Nan} output or did not attain loss below -3000}%
\end{table}

\begin{table}%
\centering%
\adjustbox{tabular=|c|c|c|c|c|, center}{
\hline%
lr&$\gamma$-Parametrization&\multicolumn{3}{|c|}{$\sigma$ Parametrization}\\%
\hline%
&&Vanilla&Exp&BoundedExp\\%
\hline%
\multirow{3}{*}{0.008}&Vanilla&($0.000 \pm 0.000$)&($0.004 \pm 0.012$)&$0.004 \pm 0.001$\\%
~&Exp&($0.000 \pm 0.000$)&($0.001 \pm 0.002$)&$0.004 \pm 0.003$\\%
~&BoundedExp&($0.000 \pm 0.000$)&($0.001 \pm 0.003$)&$0.004 \pm 0.002$\\%
\hline%
\multirow{3}{*}{0.007}&Vanilla&($0.000 \pm 0.000$)&($0.045 \pm 0.131$)&$0.003 \pm 0.002$\\%
~&Exp&($0.001 \pm 0.001$)&($0.002 \pm 0.005$)&$0.002 \pm 0.001$\\%
~&BoundedExp&($0.001 \pm 0.001$)&($0.018 \pm 0.039$)&$0.003 \pm 0.001$\\%
\hline%
\multirow{3}{*}{0.006}&Vanilla&($0.001 \pm 0.001$)&($0.002 \pm 0.001$)&$0.002 \pm 0.001$\\%
~&Exp&($0.000 \pm 0.001$)&($0.001 \pm 0.001$)&$0.002 \pm 0.001$\\%
~&BoundedExp&($0.001 \pm 0.002$)&($0.001 \pm 0.001$)&$0.003 \pm 0.001$\\%
\hline%
}
\caption{Proportion of iteration spent in an instability.}%
\end{table}

\begin{table}%
\centering%
\adjustbox{tabular=|c|c|c|c|c|, center}{
\hline%
lr&$\gamma$-Parametrization&\multicolumn{3}{|c|}{$\sigma$ Parametrization}\\%
\hline%
&&Vanilla&Exp&BoundedExp\\%
\hline%
\multirow{3}{*}{0.008}&Vanilla&($0.000 \pm 0.000$)&($inf \pm nan$)&$0.007 \pm 0.008$\\%
~&Exp&($0.000 \pm 0.000$)&($inf \pm nan$)&$0.016 \pm 0.023$\\%
~&BoundedExp&($0.000 \pm 0.000$)&($519835568465510.500 \pm 1559506705396531.500$)&$0.012 \pm 0.017$\\%
\hline%
\multirow{3}{*}{0.007}&Vanilla&($0.000 \pm 0.000$)&($3411042.803 \pm 10233128.399$)&$0.007 \pm 0.009$\\%
~&Exp&($0.001 \pm 0.002$)&($inf \pm nan$)&$0.003 \pm 0.002$\\%
~&BoundedExp&($0.001 \pm 0.003$)&($2957213217802003415040.000 \pm 8780030332475899117568.000$)&$0.003 \pm 0.002$\\%
\hline%
\multirow{3}{*}{0.006}&Vanilla&($0.001 \pm 0.002$)&($inf \pm nan$)&$0.003 \pm 0.001$\\%
~&Exp&($0.001 \pm 0.004$)&($0.001 \pm 0.001$)&$0.003 \pm 0.002$\\%
~&BoundedExp&($0.002 \pm 0.003$)&($0.001 \pm 0.001$)&$0.003 \pm 0.002$\\%
\hline%
}
\caption{Mean value of max(Z-4, 0) where Z is the standard Z score measured with the smoothed mean and std values}%
\end{table}
